# Supplementary material for: Weakly Supervised Contrastive Learning
Source: arXiv:2110.04770 source file (2021-10-10)
Supplement: Supplementary file 1 [file supplementary.tex]

\section{Effect of Hyper Parameters}
In previous experiments, we simply give the equal weight to  $\mathcal{L}_{swap}$ and $\mathcal{L}_{NCE}$ since they are the same type of loss. (According to Eq \eqref{equation:swap_ce}, $\mathcal{L}_{swap}$ will be added twice, hence $\beta=0.5$ actually gives the equal weight.) Now, we did some additional experiments to explore the optimal $\beta$. The result is shown in Table \ref{table:beta}. Surprisingly, $\beta=0.5$ is indeed the optimal choice for $\beta$.

\begin{table}[h]
 \vspace{-7pt}
 \centering
 \small
 \caption{Effect of $\beta$ (ImageNet100)}
 \label{table:beta}
\begin{tabular}{c | c | c | c | c | c  } 
\hline
$\beta$ & 0.125 & 0.25 & 0.5 & 0.75 & 1.0 \\
\hline
Accuracy &  76.79 & 76.91 & \textbf{77.51} & 76.95 & 76.09 \\
\hline
\end{tabular}
\vspace{-10pt}
\end{table}

\section{Visualization of Connected Components}
To further demonstrate the effectiveness of the auxiliary projection head, we randomly select 4096 images from ImageNet and perform the CCL process on the embeddings. We find out the number of connected components is always around 850 to 950, which is very close to the number of classes in the ImageNet dataset. We also show some CCL results below. As we can see, our proposed auxiliary projection head can effectively find the semantic similar samples via CCL process.

\begin{figure*}[b]
    \vspace{-10pt}
    \centering
    \label{fig:ccl_show}
    \includegraphics[width=0.85\linewidth]{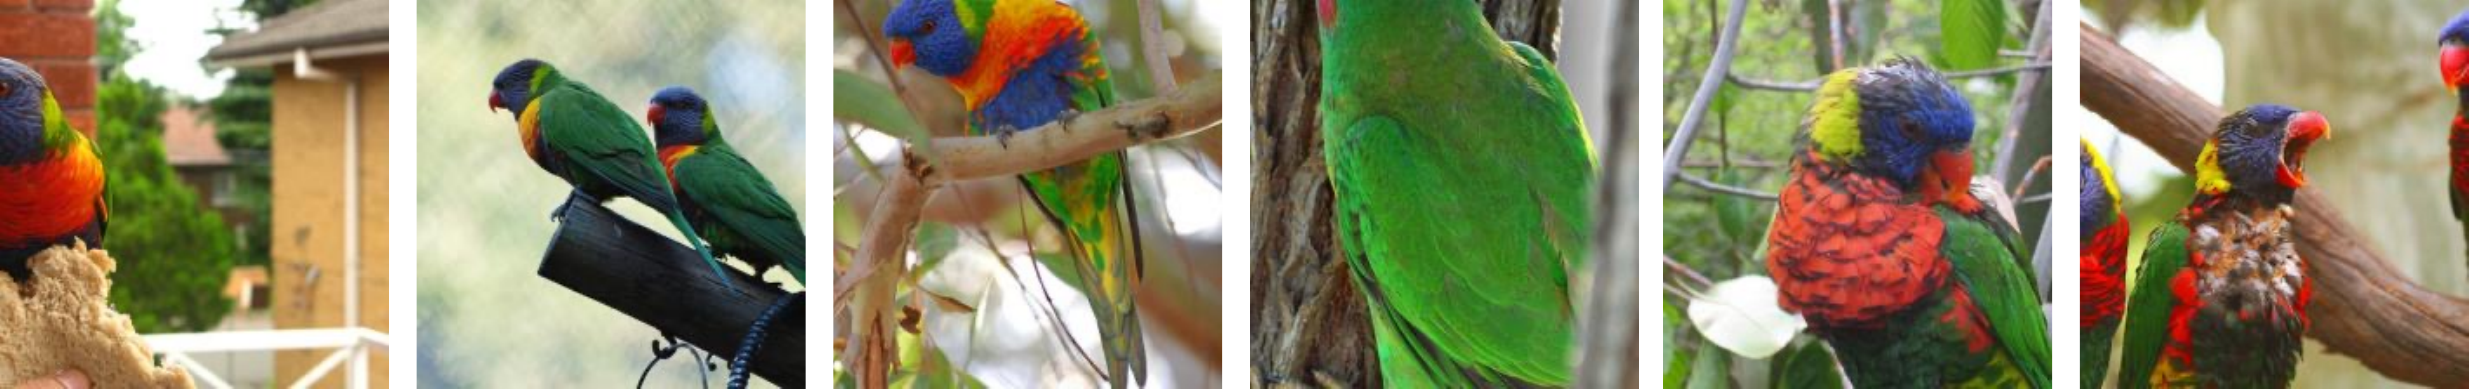} \\
    \vspace{4pt}
    \includegraphics[width=0.85\linewidth]{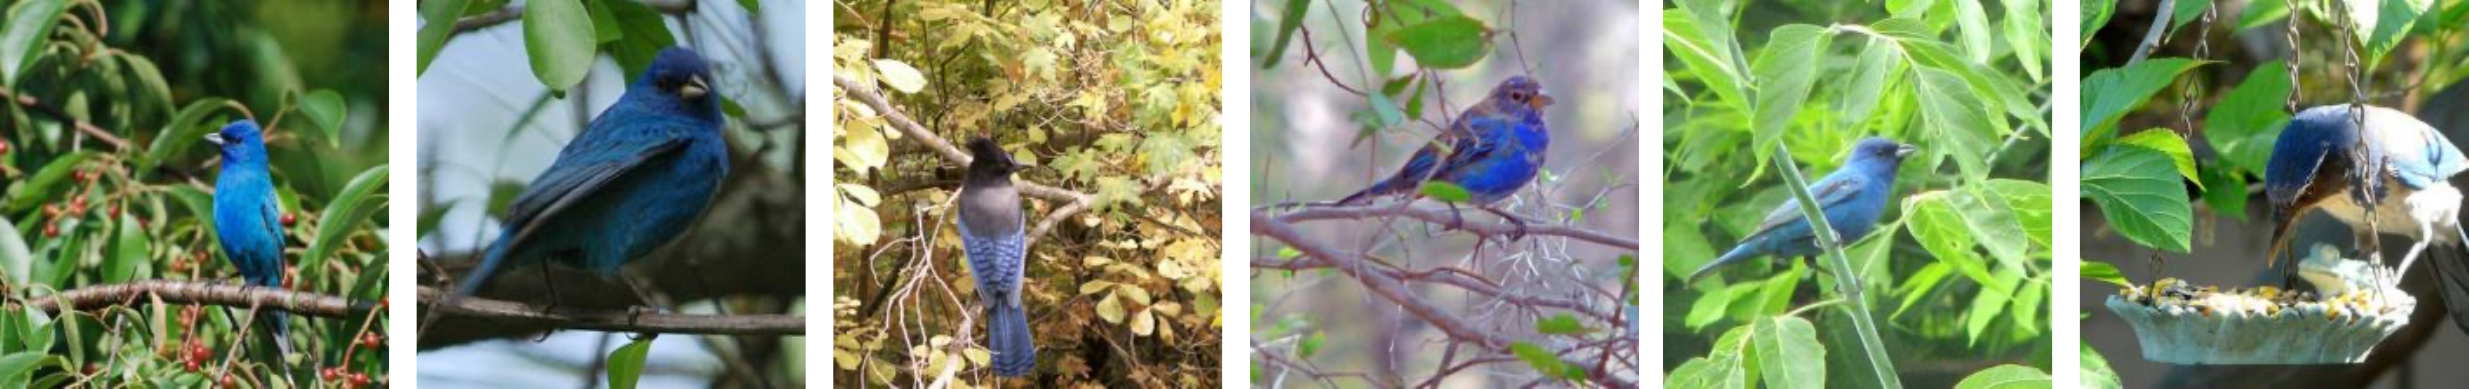} \\
    \vspace{4pt}
    \includegraphics[width=0.85\linewidth]{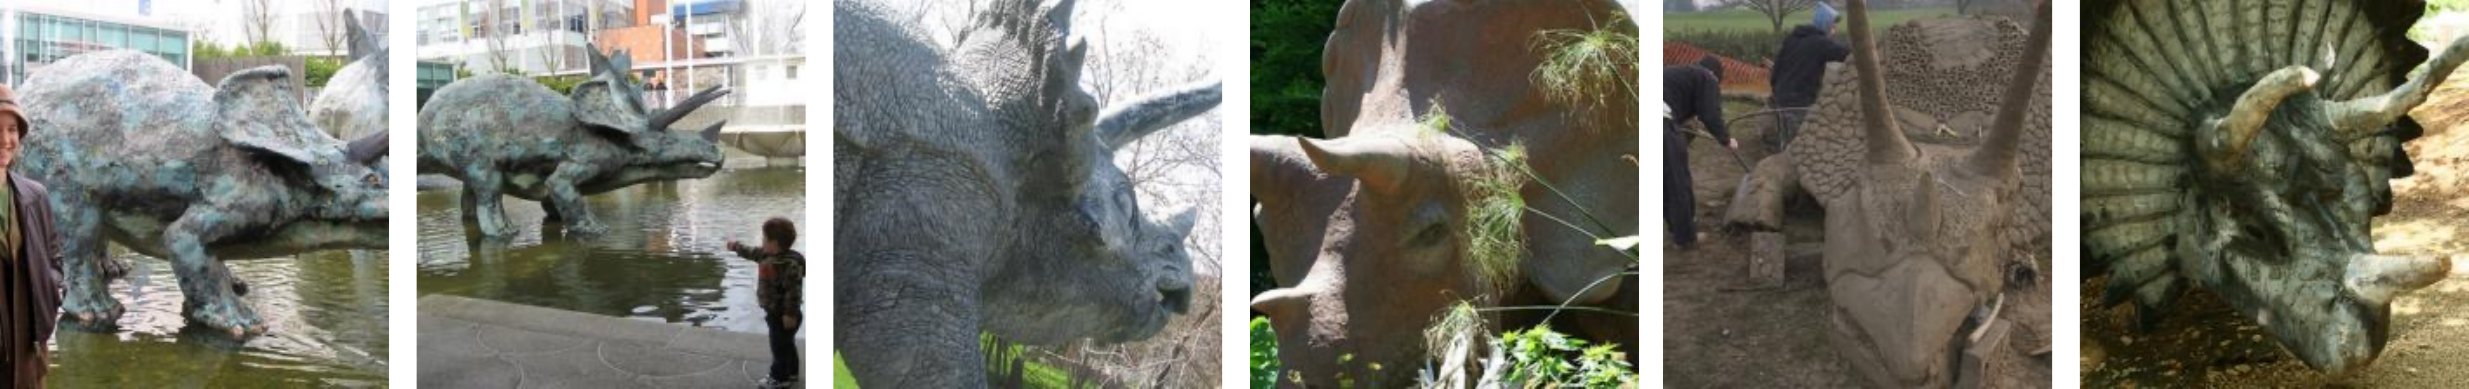} \\
    \vspace{4pt}
    \includegraphics[width=0.85\linewidth]{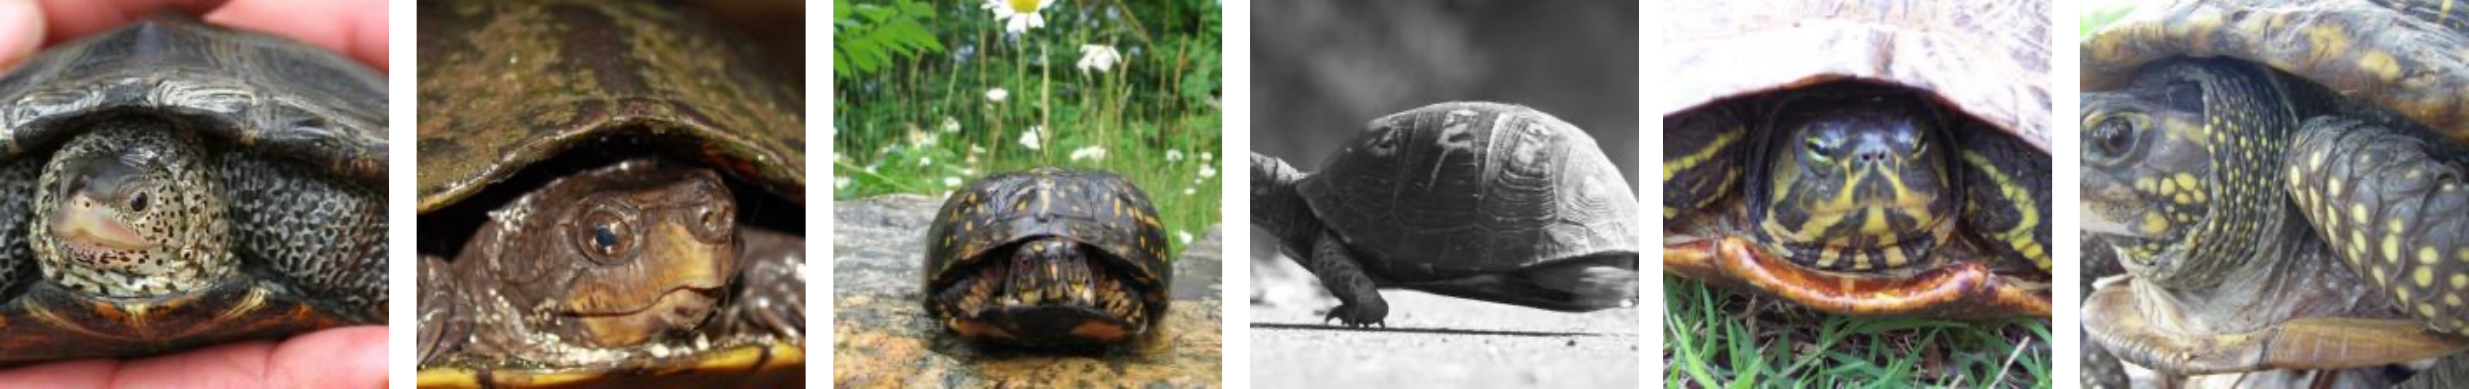} \\
    \vspace{4pt}
    \includegraphics[width=0.85\linewidth]{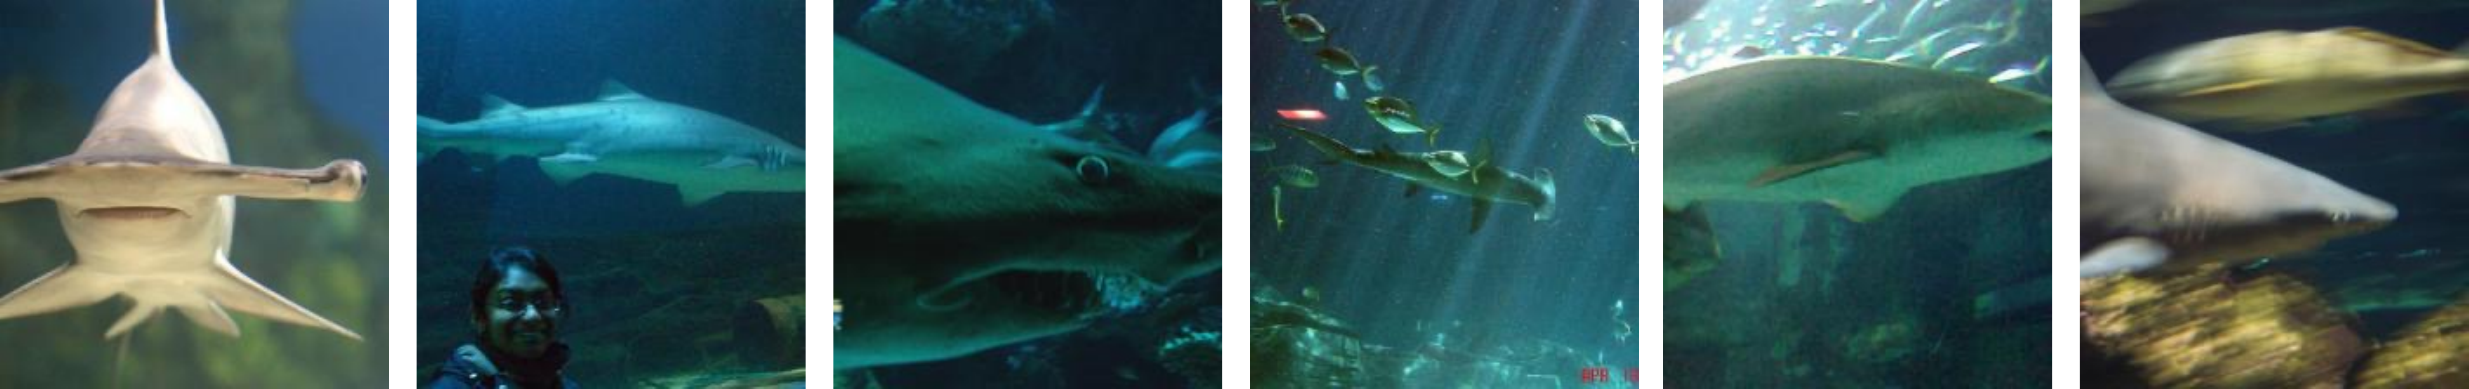} \\
    \vspace{4pt}
    \includegraphics[width=0.85\linewidth]{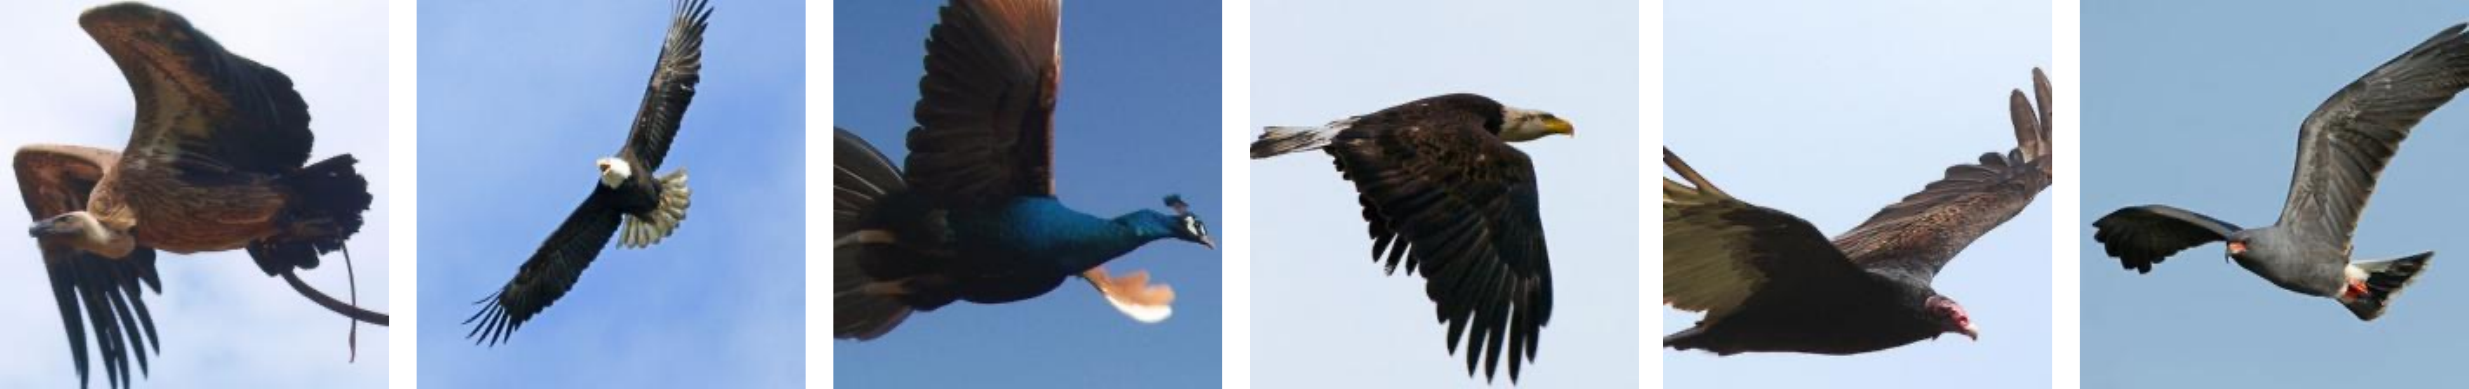} \\
    \caption{Some CCL results. Images in the same row belong to the same connected components}
\end{figure*}
